# Supplementary material for: Multi-granularity Interest Retrieval and Refinement Network for Long-Term User Behavior Modeling in CTR Prediction
Source: arXiv:2411.15005 source file (2025-02-17)
Supplement: Supplementary file 1 [file appendix.tex]

\label{appendix:datasets}

\section{Further Experimental Results}

\begin{figure}[h]
% \begin{figure}[t]
  \centering
  \includegraphics[width=\linewidth]{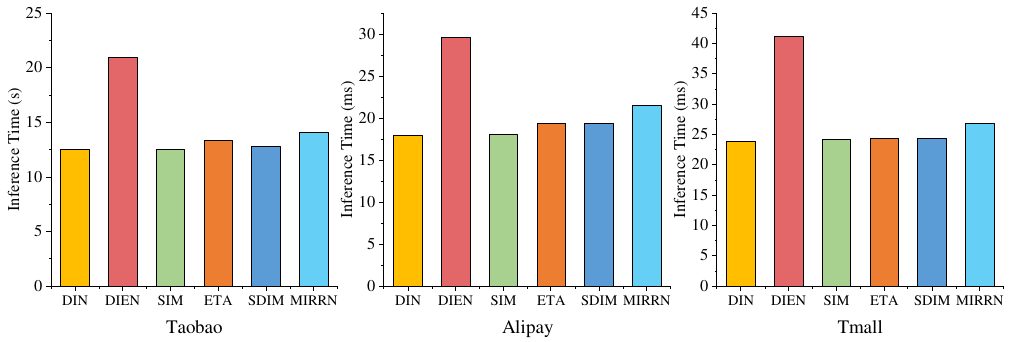}
  \caption{The Inference Time}
  \label{fig:time}
  \Description{}
\end{figure}

\begin{figure}[t]
% \begin{figure}[t]
  \centering
  \includegraphics[width=0.5\linewidth]{./figure/Graph1.pdf}
  \caption{The Inference Time}
  \label{fig:time}
  \Description{}
\end{figure}
\begin{figure}[t]
% \begin{figure}[t]
  \centering
  \includegraphics[width=0.5\linewidth]{./figure/Graph2.pdf}
  \caption{The Inference Time}
  \label{fig:time}
  \Description{}
\end{figure}
\begin{figure}[t]
% \begin{figure}[t]
  \centering
  \includegraphics[width=0.5\linewidth]{./figure/Graph3.pdf}
  \caption{The Inference Time}
  \label{fig:time}
  \Description{}
\end{figure}
